# Supplementary material for: Minimize Quantization Output Error with Bias Compensation
Source: arXiv:2404.01892 source file (2024-04-02)
Supplement: Supplementary file 1 [file 08-Appendix.tex]

\section{Appendix}
